# Supplementary material for: Monitoring Critical Infrastructure Facilities During Disasters Using Large Language Models
Source: arXiv:2404.14432 source file (2024-04-18)
Supplement: Supplementary file 1 [file appendix.tex]

\section{Appendix}
\label{sec:appendix}
\begin{table}[hbt!]
\centering
\caption{\label{broward_cifs}CIFs utilized for Broward County}
% \begin{tabular}{|c|c|c|}
\begin{adjustbox}{max width=\linewidth}
\begin{tabular}{lll}
\toprule
\textbf{Fire Stations}                       & Westside Regional Medical Center Emergency & Sagemont Upper School                                     \\
Broward County Fire / Rescue Station 106     & Icon Medical Centers                                         & The Sagemont Upper School                                 \\
Pembroke Pines Fire / Rescue Station 69      & Samuel Freedman M.D.                                         & Gator Run Elementary School                               \\
Miramar Fire Rescue Station 70               & Memorial Pembroke 24/7 Care Center                           & New Renaissance Middle School                             \\
Miramar Fire Rescue Station 107              & East Medical Plaza                                           & Project School                                            \\
Fire Station Number 88                       & Central Medical Plaza                                        & La Peptite of Miramar                                     \\
Fire Station 53                              & North Medical Plaza                                          & Broward College South Campus                              \\
Pompano Beach Fire Prevention                & MD Now Urgent Care                                           & Miami Dade College Learning Center                        \\
Coconut Creek Fire Department                & Matthew Taub Mdpa                                            & Concorde Career Institute - Miramar                       \\
Honey Hill Fire Department Station 51        & Kidney Doctor's Dialysis Centers                             & Broward College - North Campus                            \\
Honey Hill Fire Station                      & Marshal E. Lieberfarb, MD, PhD                               & Broward College                                           \\
Carol City Fire Department Station 11        & Century Oncology Radiation Therapy                           & Florida Atlantic University, Davie Campus \\
\textbf{Medical Facilities}                  & 21st Century Oncology                                        & University of Florida Field Laboratory                    \\
South Florida State Hospital                 & Broward Outpatient Medical Center                            & Nova Southeastern University                              \\
Kindred Hospital South Florida - Hollywood   & \textbf{Educational Facilities}                              & University of Phoenix                                     \\
Memorial Regional Hospital                   & Saint Gregory School                                         & DeVry University                                          \\
Memorial Hospital Pembroke                   & Saint Bartholomew School                                     & Keiser College                                            \\
Plantation General Hospital                  & South Area Alternative School                                & \textbf{Airports/Aerodromes}                                         \\
Aventura Hospital and Medical Center         & Hallandale High School                                       & North Perry Airport                                       \\
Westside Regional Medical Center             & ATA Flight School                                            & Fort Lauderdale Executive Airport                         \\
Hollywood Medical Center                     & Annunciation School                                          & Pompano Beach Airpark                                     \\
Holy Cross Hospital                          & Orange Brook School                                          & \textbf{Bridges, Tunnels, Railway Stations}               \\
Memorial Hospital West                       & Sunshine Elementary School                                   & Armagh Street Bridge                                                    \\
Broward Health North                         & Dolphin Park High School                                     & Southeast 6th Avenue Station                                      \\
Broward Health Imperial Point                & Beth Shalem Day School                                       & Hollywood Station                                                 \\
Fort Lauderdale Behavioral Health Center     & Sea Castle Elementary School                                 & Sheridan Street Station                                         \\
Northwest Medical Center                     & Miramar High School                                          & Aventura Station                                                 \\
Passport Health Pembroke Pines Travel Clinic & Cambridge Schools in Weston                                  & Pompano Beach Station                                          \\
Passport Health Ft. Lauderdale Travel Clinic & North Point School                                           & Cypress Creek Station\\
\bottomrule
\end{tabular}
\end{adjustbox}
\end{table}

\begin{table}[hbt!]
\caption{\label{christchurch_cifs}CIFs utilized for Christchurch}
\begin{adjustbox}{max width=\linewidth}
\begin{tabular}{lll}
\toprule
\textbf{Fire Station}                  & High Street City Health                & Riccarton High School                     \\
Christchurch City Fire Station         & Straven Medical                        & The Cathedral Grammar School              \\
Christchurch International Airport RFS & Ear Health Riccarton                   & Saint Thomas of Canterbury College        \\
Spreydon Fire Station                  & Barrington Medical Centre              & Breens Intermediate School                \\
Ilam Fire Station                      & Etu Pasifika                           & Catholic Cathedral College                \\
Harewood Fire Station                  & Integrated Health Care                 & Villa Maria College                       \\
Wigram Fire Station                    & Health \& Sport Central                & Christchurch College of English           \\
Redwood Fire Station                   & Maui Clinic                            & New Zealand College of Business           \\
Sumner Volunteer Fire Brigade          & Triton Hearing Clinic, St Albans       & New Zealand Broadcasting School           \\
\textbf{Medical Facilities}            & Triton Hearing Clinic, Papanui         & University of Otago Christchurch Campus   \\
Christchurch Hospital                  & Riccarton Clinic                       & MAINZ Christchurch                        \\
Christchurch Public Hospital           & Triton Hearing                & University of Canterbury                  \\
Christchurch Outpatients               & \textbf{Educational Facilities}        & School of Medicine                        \\
Southern Cross Hospital                & Christchurch Girls' High School        & Ara Institute of Canterbury               \\
Hillmorton Hospital                    & Christchurch Boys' High School         & JZ - Tai Haruru                           \\
Canterbury Charity Hospital            & Christchurch South Intermediate School & \textbf{Airports/Aerodrome}                         \\
Youth Specialty Services               & Christchurch East School               & Christchurch International Airport        \\
Regional Forensic Psychiatric Service  & Christchurch Adventist School          & Former Wigram Aerodrome Apron and Taxi \\
The Cosmetic Clinic                    & Christchurch Rudolf Steiner School     & Former Wigram Aerodrome                   \\
Sexual Health Clinic                   & Christ's College                       & \textbf{Railway Stations}                 \\
The Merivale Clinic                    & Middleton Grange School                & Christchurch Station \\
\bottomrule
\end{tabular}
\end{adjustbox}
\end{table}
